# Supplementary material for: Robust Stochastically-Descending Unrolled Networks
Source: arXiv:2312.15788 source file (2024-11-29)
Supplement: Supplementary file 1 [file appendix.tex]

\section{Preliminaries in Galois-Field Theory}

\section{Proofs}
